# Supplementary material for: Enhancing Offline Reinforcement Learning with Curriculum Learning-Based Trajectory Valuation
Source: arXiv:2502.00601 source file (2025-04-13)
Supplement: Supplementary file 1 [file limitations.tex]

\section{Limitations}
\label{sec-limitations}

\textbf{Parameters of TS:}
\begin{itemize}
    \item Our TS method can be further improved by using an adaptive mechanism for the TS parameters $\delta$ and $\lambda$, representing the ratio of transition similarity to the reward of TS, and the ratio of transition score to transition reward, respectively.
\end{itemize}
\textbf{Performance of CLTV:}
\begin{itemize}
    \item Transition Scoring (TS) method is limited to the environments that share the same state and action spaces across source and target domains, as we have shown in our work. This restricts the generalizability of our approach to domains with different state and action spaces.
    \item While our CLTV method significantly improves offline RL methods, finding the optimal number of selected trajectories for curriculum learning is challenging. This number must be experimentally determined for each task, requiring multiple attempts to ensure it fits the specific scenarios. This process can be both time-consuming and resource-intensive.
    \item Calculating the value of each trajectory can be computationally expensive, particularly with a large number of trajectories. This can limit the scalability of our approach when applied to larger datasets or more complex environments.
\end{itemize}
