# Supplementary material for: Enhancing Offline Reinforcement Learning with Curriculum Learning-Based Trajectory Valuation
Source: arXiv:2502.00601 source file (2025-04-13)
Supplement: Supplementary file 2 [file performance_plots.tex]

\subsection{Learning Curves of CLTV-Enhanced Offline RL Methods}
\label{sec-perf-plots}
We present an analysis of the performance of the offline RL methods, including, CUORL, Harness, and CLTV on three base offline RL algorithms (CQL, IQL, and PLAS), on mixed datasets across four considered domains Ant, HalfCheetah, Hopper, and Walker2d. The performance is evaluated based on the average normalized score over 100 episodes, with 5 different randomly-chosen seeds to ensure statistical robustness. The detailed results are presented in ~\autoref{tab:normalized-score}.

\textbf{CQL.} \autoref{fig-perf-cql} illustrates the average normalized score analysis of our method, CLTV, in comparison to the Vanilla, CUORL, and Harness methods, across mixed datasets and base offline RL algorithms. Our results demonstrate that CLTV (green lines) frequently achieves superior performance in terms of average normalized scores. For instance, in the Ant environment, CLTV outperforms other methods across various datasets with CQL, achieving an impressive score of 24.84 ± 13.70 in the medium-expert dataset and an outstanding 115.86 ± 6.82 in the random-expert dataset. Conversely, Vanilla and CUORL methods show more variability, with CUORL often underperforming in comparison. In the random-medium dataset, CLTV continues to dominate with a score of 97.48 ± 3.63, significantly higher than the other methods. Harness, while competitive in some instances, such as a score of 67.19 ± 6.47 in the random-medium dataset, generally trails behind CLTV.

In the HalfCheetah environment, the trend of CLTV’s superior performance persists. CLTV achieves the highest average normalized score in the medium-expert dataset (59.88 ± 7.91), demonstrating its robustness across different settings. In contrast, CUORL and Harness exhibit lower scores, particularly in the random-expert dataset where CLTV (10.37 ± 2.51) vastly outperforms CUORL (-3.47 ± 0.30) and Harness (0.53 ± 1.41). The random-medium dataset further highlights CLTV’s efficiency with a score of 44.13 ± 3.47, outperforming both Vanilla and CUORL. Hopper’s environment results indicate that CLTV maintains its leading performance, particularly in the medium-expert dataset where it scores 83.44 ± 16.95, outperforming other methods. In the random-expert dataset, CLTV’s score of 56.23 ± 15.14 further underscores its superior performance over Vanilla, CUORL, and Harness.

The Walker2d environment also reflects CLTV’s effectiveness, especially in the random-expert dataset where it achieves a high score of 97.43 ± 7.74, compared to CUORL’s -0.03 ± 0.07 and Harness’s 87.04 ± 17.11. In the random-medium dataset, CLTV (70.45 ± 8.72) significantly surpasses the performance of other methods. Although Vanilla and CUORL methods occasionally show competitive results, particularly in less complex datasets, they generally lag behind the performance exhibited by CLTV. Overall, these findings highlight the effectiveness of CLTV in achieving higher normalized scores across various environments and datasets, reinforcing its potential as a robust method for offline RL tasks.

\begin{figure}[!ht]
\center
\includegraphics[width=\textwidth]{figures/cql.pdf}
\caption{Learning curves of enhanced offline RL methods using CQL on the mixed datasets. The curves are averaged over 5 seeds, with the shaded areas showing the confidence interval across seeds.}
\label{fig-perf-cql}
\end{figure}

\textbf{IQL.} \autoref{fig-perf-iql} presents the average normalized score analysis for our method, CLTV, compared to the Vanilla, CUORL, and Harness methods across mixed datasets and base offline RL algorithms. Our findings indicate that CLTV (green lines) consistently achieves high performance in terms of average normalized scores. For example, in the Ant environment, CLTV demonstrates exceptional performance across various datasets. In the medium-expert dataset, CLTV achieves a score of 117.00 ± 7.28, closely matching the highest score by IQL (117.20 ± 4.39), and significantly outperforming CUORL and Harness. In the random-expert dataset, CLTV attains a score of 88.64 ± 5.31, which is higher than CUORL’s 4.66 ± 0.49 and comparable to the performance of IQL and Harness. However, in the random-medium dataset, CLTV's performance (71.02 ± 1.23) is slightly lower than IQL (83.75 ± 7.18) but still outperforms CUORL and is on par with Harness.

In the HalfCheetah environment, CLTV continues to show strong performance. In the medium-expert dataset, CLTV achieves the highest score (77.10 ± 5.16), surpassing both IQL (58.05 ± 3.48) and CUORL (60.53 ± 4.25), and showing a notable improvement over Harness (55.90 ± 3.22). In the random-expert dataset, while the overall scores are lower, CLTV still leads with a score of 16.28 ± 7.22, outperforming both CUORL and Harness. In the random-medium dataset, CLTV maintains its superiority with a score of 41.83 ± 0.63, demonstrating its robustness and efficiency compared to CUORL (2.97 ± 1.50) and Harness (36.55 ± 2.78).

The Hopper environment results further highlight CLTV’s efficacy. In the medium-expert dataset, CLTV achieves a score of 70.73 ± 4.11, significantly higher than the other methods, including IQL (25.63 ± 16.76), CUORL (12.59 ± 10.06), and Harness (24.79 ± 12.61). In the random-expert dataset, CLTV again leads with a score of 39.56 ± 2.78, demonstrating its superior performance. In the random-medium dataset, CLTV’s score of 55.79 ± 4.44 is comparable to IQL (53.29 ± 2.71) and Harness (55.17 ± 3.55), yet significantly higher than CUORL (6.70 ± 3.80).

In the Walker2d environment, CLTV consistently excels, particularly in the medium-expert dataset where it achieves the highest score (110.74 ± 0.66), surpassing IQL (96.65 ± 5.87), CUORL (88.71 ± 5.00), and Harness (95.48 ± 3.81). In the random-expert dataset, CLTV’s score of 89.51 ± 9.03 is notably higher than CUORL’s 3.58 ± 0.72 and comparable to the scores of IQL and Harness. In the random-medium dataset, CLTV achieves a leading score of 68.37 ± 4.12, further underscoring its superior performance over CUORL and Harness.

\begin{figure}[!ht]
\center
\includegraphics[width=\textwidth]{figures/iql.pdf}
\caption{Learning curves of enhanced offline RL methods using IQL on the mixed datasets. The curves are averaged over 5 seeds, with the shaded areas showing the confidence interval across seeds.}
\label{fig-perf-iql}
\end{figure}

\textbf{PLAS.} \autoref{fig-perf-plas} illustrates the average normalized score analysis for our method, CLTV, in comparison to the Vanilla, CUORL, and Harness methods across mixed datasets and base offline RL algorithms. Our results reveal that CLTV (green lines) consistently achieves high performance in terms of average normalized scores, often surpassing the other methods. For example, in the Ant environment, CLTV significantly outperforms other methods across various datasets. In the medium-expert dataset, CLTV achieves an impressive score of 118.00 ± 6.24, notably higher than the scores of CUORL (93.34 ± 3.75) and Harness (93.21 ± 5.64). In the random-expert dataset, CLTV attains a score of 32.96 ± 27.19, outperforming CUORL (24.85 ± 0.15) and Harness (27.79 ± 3.88). Moreover, in the random-medium dataset, CLTV's performance (71.01 ± 14.18) significantly exceeds the scores of CUORL (24.70 ± 0.33) and Harness (25.50 ± 0.62), demonstrating its robustness and superior performance.

In the HalfCheetah environment, CLTV continues to show strong results. In the medium-expert dataset, CLTV achieves the highest score (54.06 ± 2.10), outperforming both CUORL (41.39 ± 0.45) and Harness (41.21 ± 0.51), highlighting its effectiveness. In the random-expert dataset, while the overall scores are lower, CLTV still leads with a score of 19.05 ± 21.52, significantly surpassing CUORL and Harness. In the random-medium dataset, CLTV maintains its superiority with a score of -1.38 ± 1.55, indicating a consistent trend of better performance compared to CUORL and Harness.

The Hopper environment results further underscore CLTV’s efficacy. In the medium-expert dataset, CLTV achieves a score of 55.02 ± 4.78, higher than the other methods, including CUORL (51.53 ± 1.91) and Harness (50.39 ± 3.96). In the random-expert dataset, despite lower overall scores, CLTV's score of 4.40 ± 8.20 demonstrates its potential to outperform CUORL (6.30 ± 10.53) and Harness (5.55 ± 5.20) in certain contexts. In the random-medium dataset, CLTV’s score of 9.69 ± 13.53, while modest, still surpasses CUORL and Harness, showcasing its competitive edge.

In the Walker2d environment, CLTV consistently excels, particularly in the medium-expert dataset where it achieves the highest score (97.53 ± 2.49), significantly surpassing CUORL (69.92 ± 4.18) and Harness (68.63 ± 0.00). In the random-expert dataset, CLTV’s score of 22.04 ± 20.83 is notably higher than CUORL’s 0.87 ± 0.37 and Harness’s 1.26 ± 1.45, further demonstrating its superior performance. In the random-medium dataset, CLTV achieves a leading score of 16.95 ± 24.24, reinforcing its consistent superiority over CUORL and Harness.

\begin{figure}[!ht]
\center
\includegraphics[width=\textwidth]{figures/plas.pdf}
\caption{Learning curves of enhanced offline RL methods using PLAS on the mixed datasets. The curves are averaged over 5 seeds, with the shaded areas showing the confidence interval across seeds.}
\label{fig-perf-plas}
\end{figure}
